# Supplementary material for: Repulsive Surfaces
Source: arXiv:2107.01664 ancillary file (2021-07-04)

IrregularTorus\_01

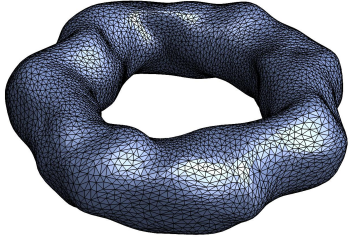

IrregularTorus\_02

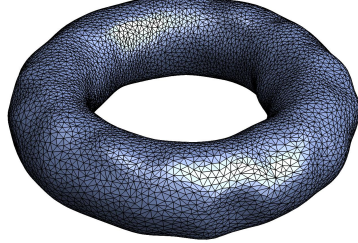

IrregularTorus\_03

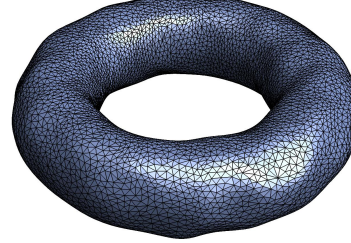

IrregularTorus\_04

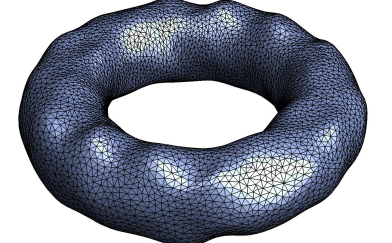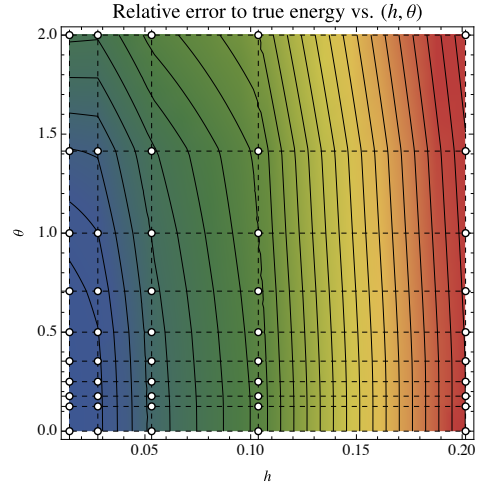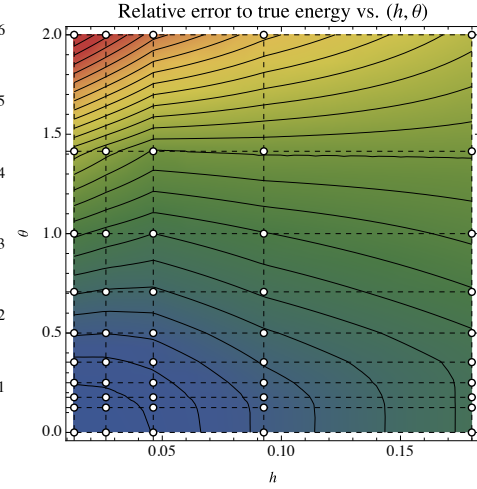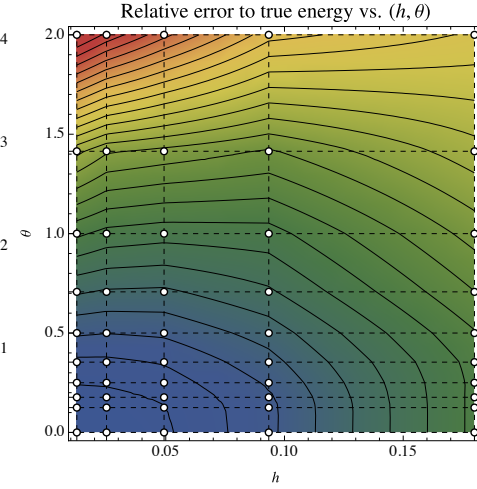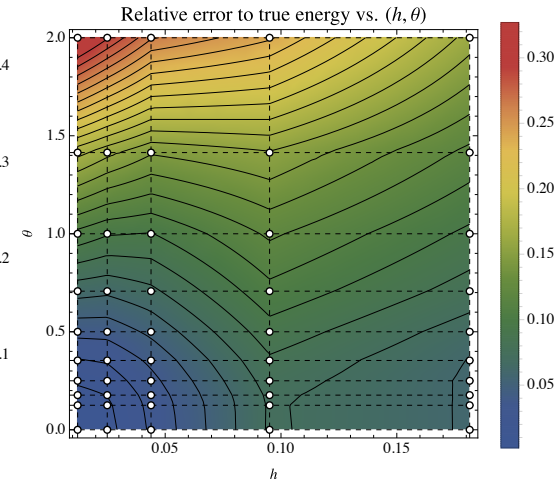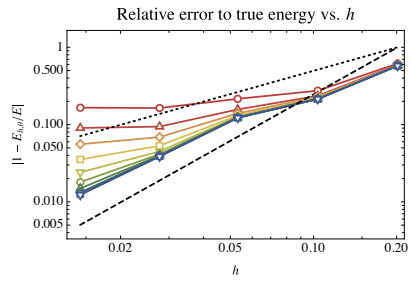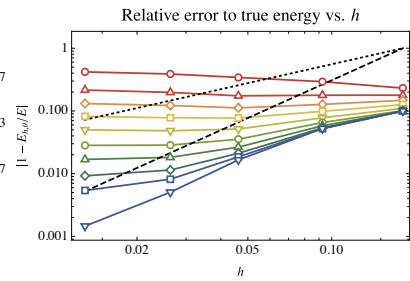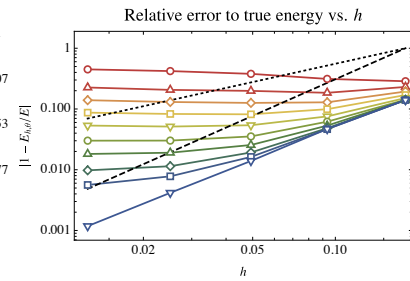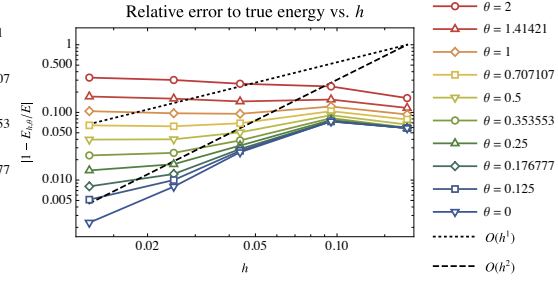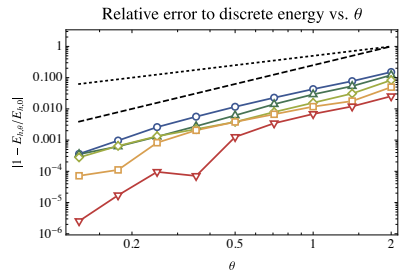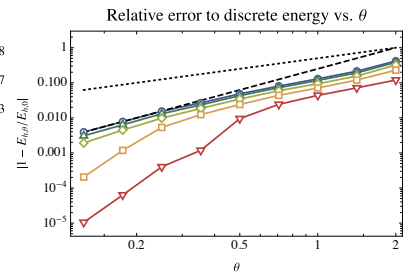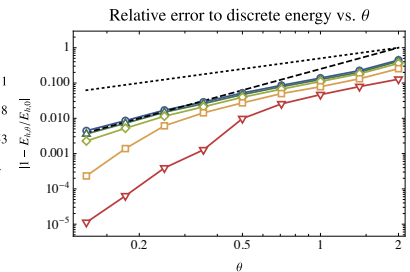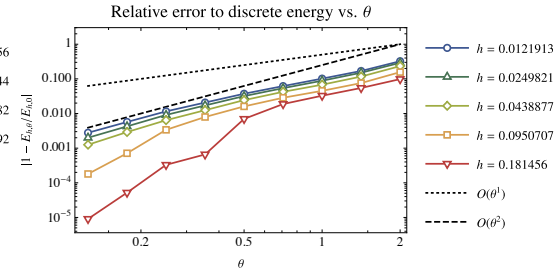

IrregularTorus\_05

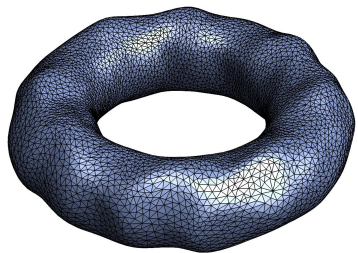

IrregularTorus\_06

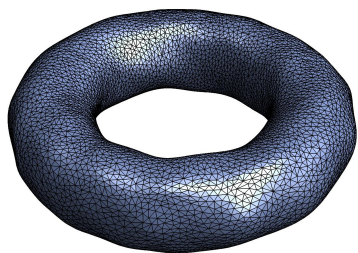

IrregularTorus\_07

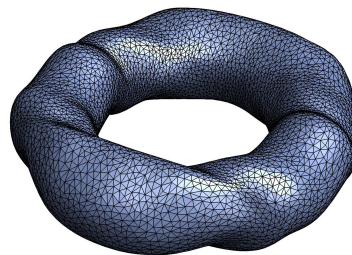

IrregularTorus\_08

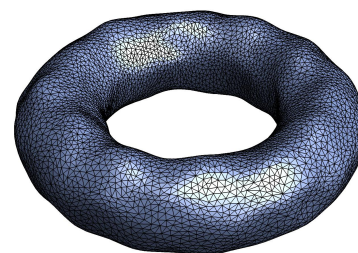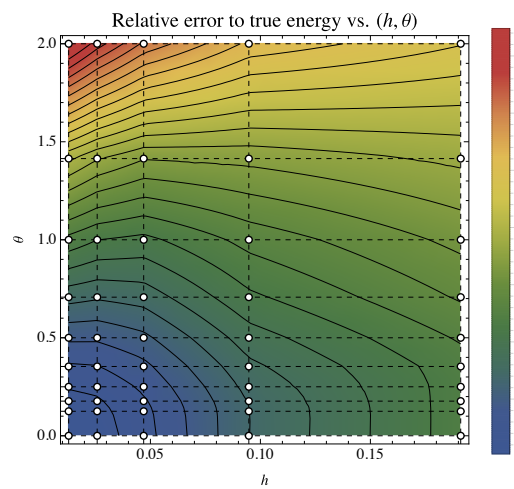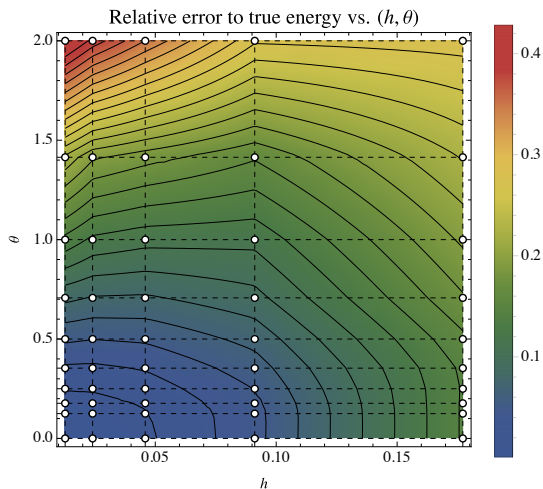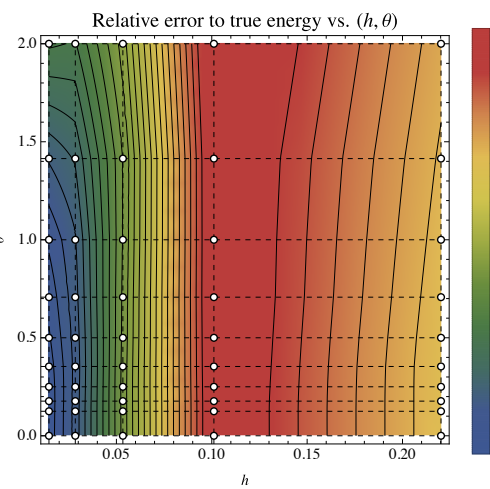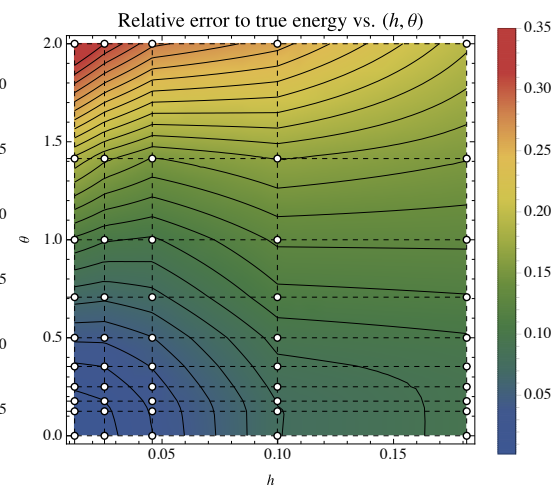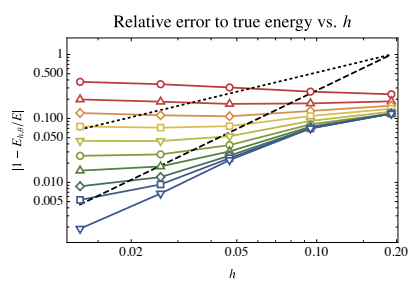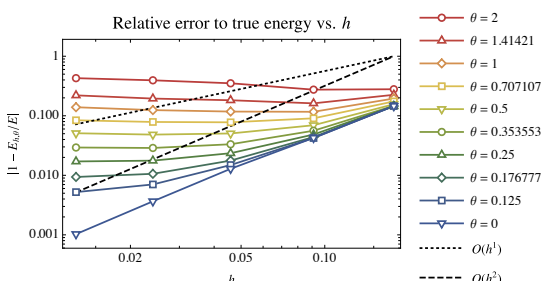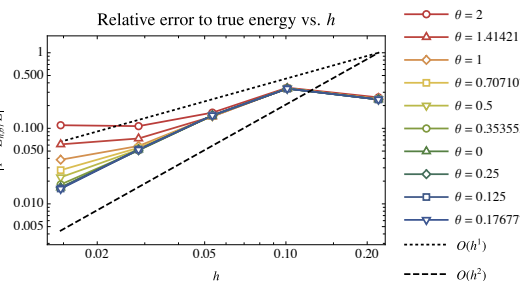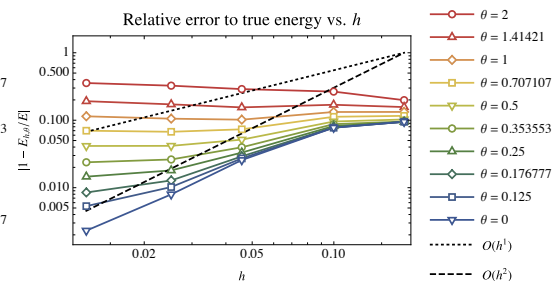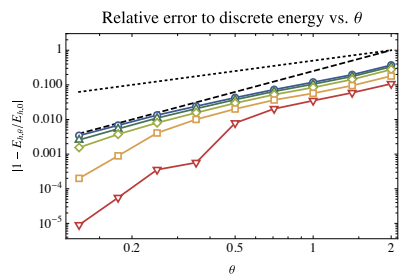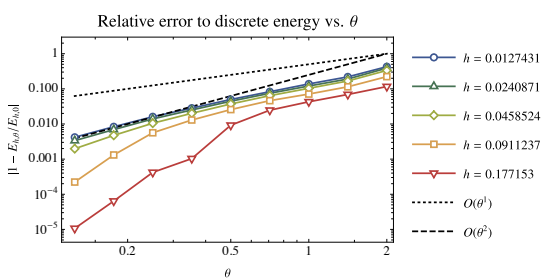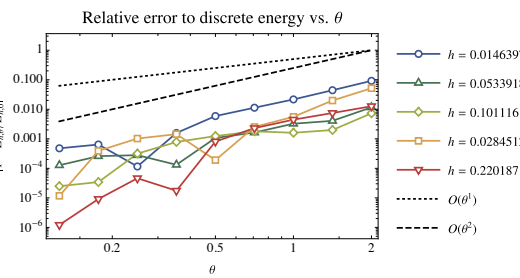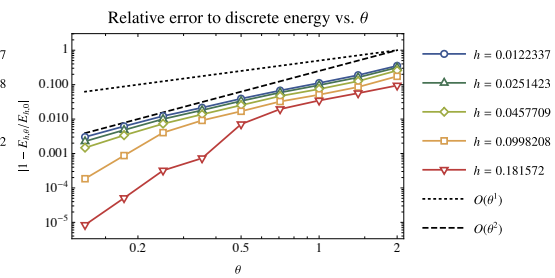

Supplement: Supplementary file 1 [file MoreConsistencyTests.pdf]
